# Supplementary material for: Robust Multi-agent Communication Based on Decentralization-Oriented Adversarial Training
Source: arXiv:2504.21278 source file (2025-04-30)
Supplement: Supplementary file 1 [file 7_appendix.tex]

\newpage
\appendix
\section{Appendix}
\label{sec:app}

\subsection{Details of Experiments}

\textbf{Experimental Environment.}
To demonstrate the generalization of {\tool}, we use three different multi-agent benchmarks for a total of four tasks to evaluate. We will introduce the settings of the three platforms. 

\textbf{SMAC.} In the SMAC, each scenario is a confrontation between two armies of units, where the allied agents are controlled by learned agents. The goal of allied agents is to defeat the enemy units controlled by the built-in AI by the obtained messages, where the rewards are related with the health value of all enemy agents and the final outcome of the battle.

\textbf{MPE.} In the MPE, the agents need to achieve the target landmarks without any collision. The reward is related with the distance between the agent and the landmark and the number of collisions. We choose two scenarios officially provided in MPE for evaluation: Coop Navi (simple\_spread) and Predator Prey (simple\_tag). In coop navi, 7 agents must cooperate through physical actions to reach a set of landmarks. Agents observe the relative positions of other agents and landmarks, and are collectively rewarded based on the proximity of any agent to each landmark. Further, the agents occupy significant physical space and are penalized when colliding with each other. Agents must learn to infer the landmark they must cover, and move there while avoiding other agents. In Predator Prey, 8 slower cooperating agents (Predator) must chase the faster adversary (Prey) around a randomly generated environment with several landmarks impeding the way. Each time the predators collide with an adversary, the predators are rewarded while the preys are penalized. 

\textbf{Traffic Junction.} In the traffic junction, 10 cars enter a junction from entry points. Cars can take two actions at each time-step, \textit{gas} and \textit{break} respectively. At each step, each agent observes its previous actions, the route identifier, and a vector that specifies the sum of the one-hot vectors of all objects present at the agent's location. A collision occurs when two vehicles are at the same location, and the agent receives a reward of -10 if a collision occurs. Additionally, to prevent traffic jams, an agent receives a negative reward of -0.01 for each time step when it is at an intersection.

\textbf{Implementation} We implement {\tool} with PyTorch. All experiments are launched on a server equipped with an NVIDIA TITAN RTX GPU, Intel Xeon Silver CPU, 64GB RAM, running on Ubuntu 20.04 OS.

\textbf{Baseline.} To evaluate the ability to identify critical communication channels, we used the following methods as baselines:

\noindent
(1) \textit{Random Attack} randomly selects and masks one communication channel at each time step without any guidance.

\noindent
(2) \textit{Reward-Based Attack} selects and masks the communication channels based on reward. Specifically, we use the reward of each agent as the basis, select the agent with the highest reward, and randomly select an agent from its neighbors, and mask the communication channel between the two agents.

\subsection{Additional Evaluations}

\begin{table}[tbp]

\centering
\caption{The win rate of the target MAS with two communication policies in four environments under various attack. The table shows three different ways to identify and attack communication connections: reward-based, random, and {\tool}. The lower the win rate, the higher the identification accuracy of critical communication connections.}
\label{tab:rq3}
\resizebox{0.5\textwidth}{!}{
\begin{tabular}{c|c|cccc} \toprule 
% & & \multicolumn{4}{c|}{\textbf{T2MAC}} & \multicolumn{4}{c}{\textbf{I2C}}  \\ \midrule 
\textbf{$CP$} &  \textbf{Attack Method}  & \textbf{SC} &  \textbf{CN} &\textbf{TJ} & \textbf{PP}   \\ \midrule 
% \textbf{Original}     & 81.2\%    & 87.4\%  & 91.7\%  & 88.6\%  & 76.9\%  & 80.1\%  & 85.2\%  & 82.4\%  \\
% \textbf{Random}     & 57.2\%  & 61.4\% & 63.6\% & 61.7\% & 51.8\% & 55.4\% & 59.3\% & 57.2\% \\

\multirow{3}{*}{\rotatebox[origin=c]{90}{\textbf{T2MAC}}} & \textbf{Reward-Based Attack}  & 37.8\%   & 40.1\%  & 55.8\%  & 47.9\%    \\
&\textbf{Random Attack} & 42.1\%  & 47.7\%  & 53.6\%  & 49.1\%    \\

&\textbf{{\tooladv}} & \textbf{16.6\% } & \textbf{19.9\% } & \textbf{34.9\% } & \textbf{26.9\%}  \\ \hline
\hline

\multirow{3}{*}{\rotatebox[origin=c]{90}{\textbf{I2C}}} & \textbf{Reward-Based Attack}   & 32.4\%  & 34.3\%  & 47.7\%  & 42.5\%  \\
& \textbf{Random Attack}  & 37.4\%  & 40.8\%   & 48.2\%  & 45.7\%  \\

& \textbf{{\tooladv}} & \textbf{12.3\% } & \textbf{14.9\% } & \textbf{30.1\% } & \textbf{22.4\% } \\

 \bottomrule
\end{tabular}}
\end{table}

\noindent
\textbf{Critical communication identification.} {As a key step towards decentralization, we evaluate the performance of the component {\tooladv}. Specifically, {\tooladv} is considered as a means of attack and compared with the other two attack methods to verify that {\tooladv} can correctly identify the most critical communication channels. }
Table \ref{tab:rq3} shows the results of different types of cutting policy. Since cutting off critical communication channels often means teams are more likely to fail, a lower win rate means more accurate identification of critical communication channels.
% \yawen{comment}
% 上面是不是跟decentralization联系上比较好，还是得说明一下这个评估的目的
As we can see, when the communication model receives perturbed from {\tooladv}, the win rate drops the most. For example, in environment SC, the original win rate of T2MAC is 81.2\% and the win rate drops to 16.6\% with {\tooladv}. However, with Heuristic-Identify, the win rate only drops to x\%, which means {\tooladv} can identify the critical communication channels more accurately.
% As for the stealthiness, the lower attack ratio, the smaller the probability of being discovered, which means the higher the stealthiness. We can see that for each communication model, in any scenario, {\tooladv} can always achieve the best attack effect with the lowest attack ratio, reflecting the effectiveness of {\tooladv}.

\begin{table}[h]

\centering
\caption{The win rate of the target MAS with two communication policies under attack in two settings. $ER$ means the \textit{embedding representation}.}
\label{tab:abl1}
\resizebox{0.5\textwidth}{!}{
\begin{tabular}{c|cccc|cccc} \toprule 
\textbf{Attack Method} & \multicolumn{4}{c|}{\textbf{Learned Adaptive Attack}} & \multicolumn{4}{c}{\textbf{Heuristic Attack}} \\ \midrule
 \diagbox{\textbf{Method}}{\textbf{Env}}& \textbf{SC} &  \textbf{CN} &\textbf{TJ} & \textbf{PP}  & \textbf{SC} &  \textbf{CN} &\textbf{TJ} & \textbf{PP} \\ \midrule 
\textbf{T2MAC+{\tool}}  & \textbf{60.4\%} & \textbf{62.7\%} & \textbf{70.4\%} & \textbf{66.3\%} & \textbf{69.9\%} & \textbf{70.1\%} & \textbf{73.8\%} & \textbf{74.4\%} \\
 \textbf{T2MAC+{\tool}-$ER$}& 49.5\%   & 50.3\%   & 58.2\%   & 48.7\%   & 51.7\%  & 59.4\% & 60.1\% & 54.0\% \\

\hline 
\hline
\textbf{I2C+{\tool}} & \textbf{58.3\%} & \textbf{59.9\%} & \textbf{67.3\%} & \textbf{62.5\%} & \textbf{66.4\%} & \textbf{68.2\%} & \textbf{70.1\%} & \textbf{71.9\%} \\
 \textbf{I2C+{\tool}-$ER$}& 40.6\% & 42.1\% & 51.0\% & 49.8\% & 46.6\% & 52.9\% & 59.9\% & 61.2\% \\

 \bottomrule
\end{tabular}}
\end{table}

\begin{table}[htbp]
\centering

\caption{The win rate of the target MAS with two communication policies in two settings. $ER$ means the \textit{embedding representation}.
% ``Original'' represents the performance of the communication model without optimization.
% \yawen{comment}
% 这个original是不是你就选了一个T2MAC作为例子，是不是T2MAC，I2C都列上啊，要不跟Table 1一样？
}
\label{tab:abl2}
\resizebox{0.45\textwidth}{!}{
\begin{tabular}{c|cccc} \toprule 
 % & \multicolumn{4}{c|}{\textbf{T2MAC}} & \multicolumn{4}{c}{\textbf{I2C}}  \\ \midrule 
\diagbox{Method}{Env}   & \textbf{SC} &  \textbf{CN} &\textbf{TJ} & \textbf{PP}  \\ \midrule

\textbf{T2MAC+{\tool}} & \textbf{83.7\%} & \textbf{89.5\%} & \textbf{93.8\%} & \textbf{90.7\%}  \\  
\textbf{T2MAC+{\tool}-$ER$} & 83.1\% & 89.0\% & 92.5\% & 89.9\%  \\  
\hline 
\hline

\textbf{I2C+{\tool}} & \textbf{79.4\%} & \textbf{83.6\%} & \textbf{90.4\%} & \textbf{88.1\%} \\

\textbf{I2C+{\tool}-$ER$} & 78.5\% & 82.4\% & 88.7\% & \86.6\%  \\  

 \bottomrule
\end{tabular}}
\end{table}

\subsubsection{Ablation Study}
As described in Section \ref{subsec:input}, the input of cutting agents contains two parts: the observation  and the embedding representation of each agent. Because using observations to generate the communication policy is a common setting, we conduct an ablation study to demonstrate the necessity of embedding representation. We compared the performance and robustness of {\tool} and w/o embedding representation (i.e., removing the embedding representation from {\tool}), as shown in Table \ref{tab:abl1} and \ref{tab:abl2}. Results show that removing \textit{embedding representation} results in decreased performance and robustness. This is because \textit{embedding representation} effectively helps {\tool} identify critical communication channels, forcing the communication policy to adjust to a decentralized mode.
